# Supplementary material for: A Space-time Model for Inferring A Susceptibility Map for An Infectious Disease
Source: arXiv:2110.09013 source file (2021-10-18)
Supplement: Supplementary file 1 [file supplement.tex]

\begin{figure*}[h!]
        \centering
        \begin{subfigure}[b]{0.475\textwidth}
            \centering
            \includegraphics[width=\textwidth, height = 0.5\textwidth]{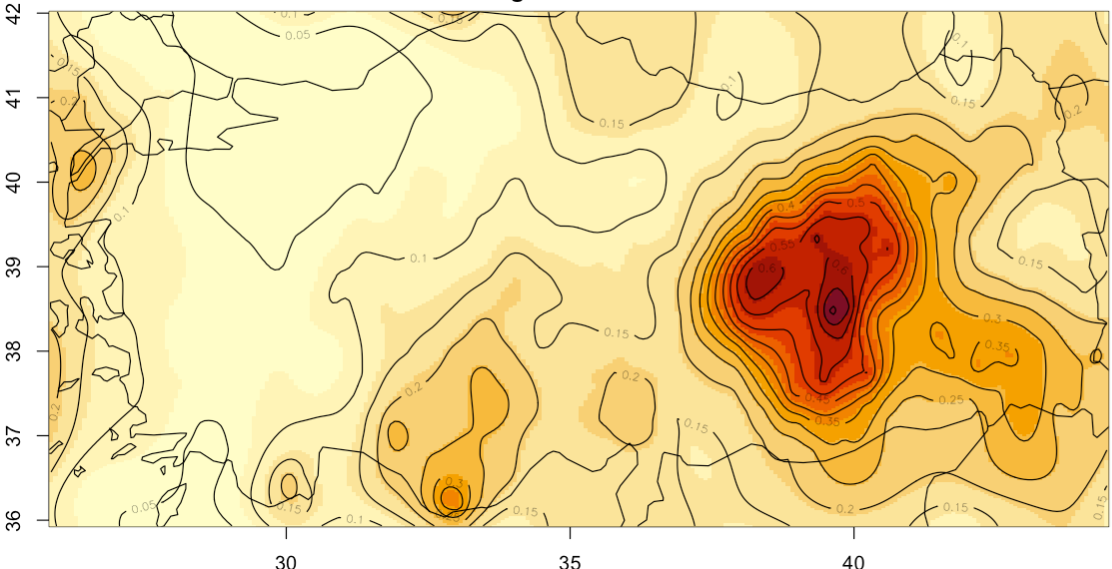}
            \caption[]{}%
            %{{\small Network 1}}    
            %\label{fig:mean and std of net14}
        \end{subfigure}
        \hfill
        \begin{subfigure}[b]{0.475\textwidth}  
            \centering 
            \includegraphics[width=\textwidth, height = 0.5\textwidth]{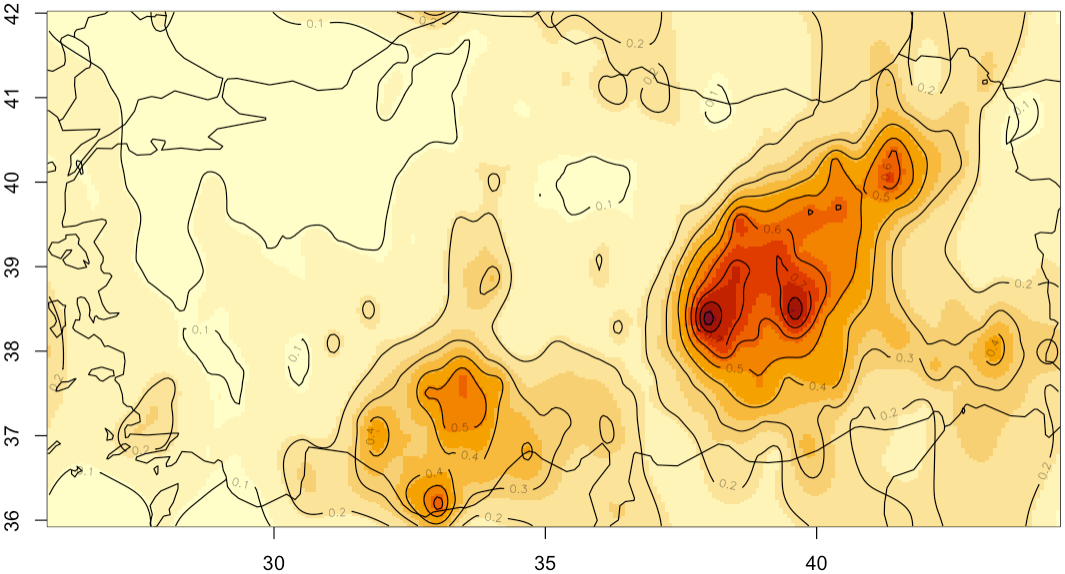}
            \caption[]{}%
           % {{\small Network 2}}    
            %\label{fig:mean and std of net24}
        \end{subfigure}
        \vskip\baselineskip
        \begin{subfigure}[b]{0.475\textwidth}   
            \centering 
            \includegraphics[width=\textwidth, height = 0.5\textwidth]{figures/fmd/sim_ground.png}
            \caption[]{}%
            %{{\small Network 3}}    
            %\label{fig:mean and std of net34}
        \end{subfigure}
        \hfill
        \begin{subfigure}[b]{0.475\textwidth}   
            \centering 
            \includegraphics[width=\textwidth, height = 0.5\textwidth]{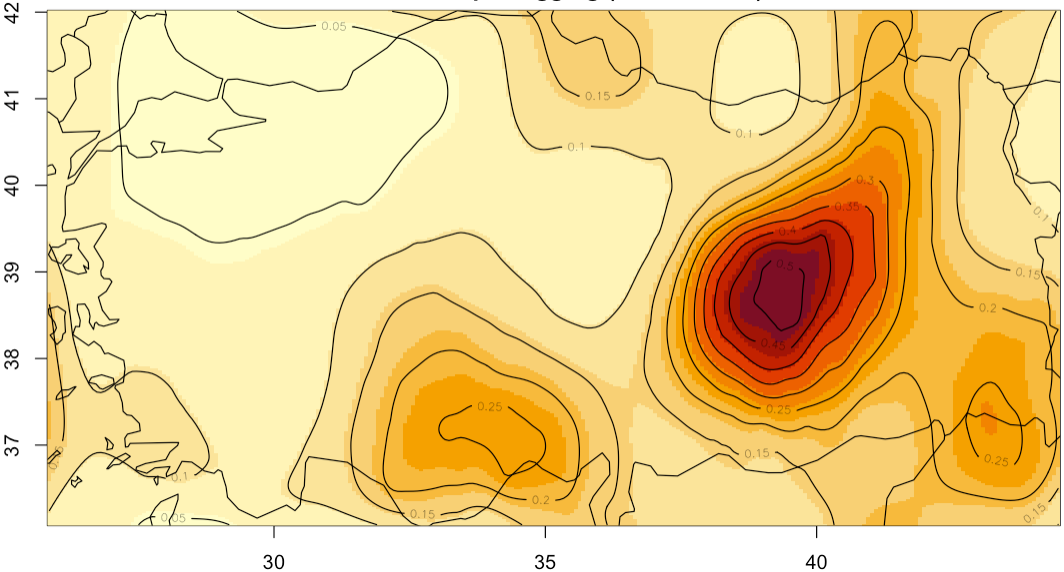}
            \caption[]{}%
            %{{\small Network 4}}    
            %\label{fig:mean and std of net44}
        \end{subfigure}
        \caption{An example of simulation study: disease risk map of susceptibility (1) ground truth of simulation experiment, and estimates inferred using (2) Model I (3) Model II (4) Model II PICAR}
        \label{fig:diseasemap}
    \end{figure*}

     \begin{figure*}
        \centering
        \begin{subfigure}[b]{0.475\textwidth}
            \centering
            \includegraphics[width=\textwidth]{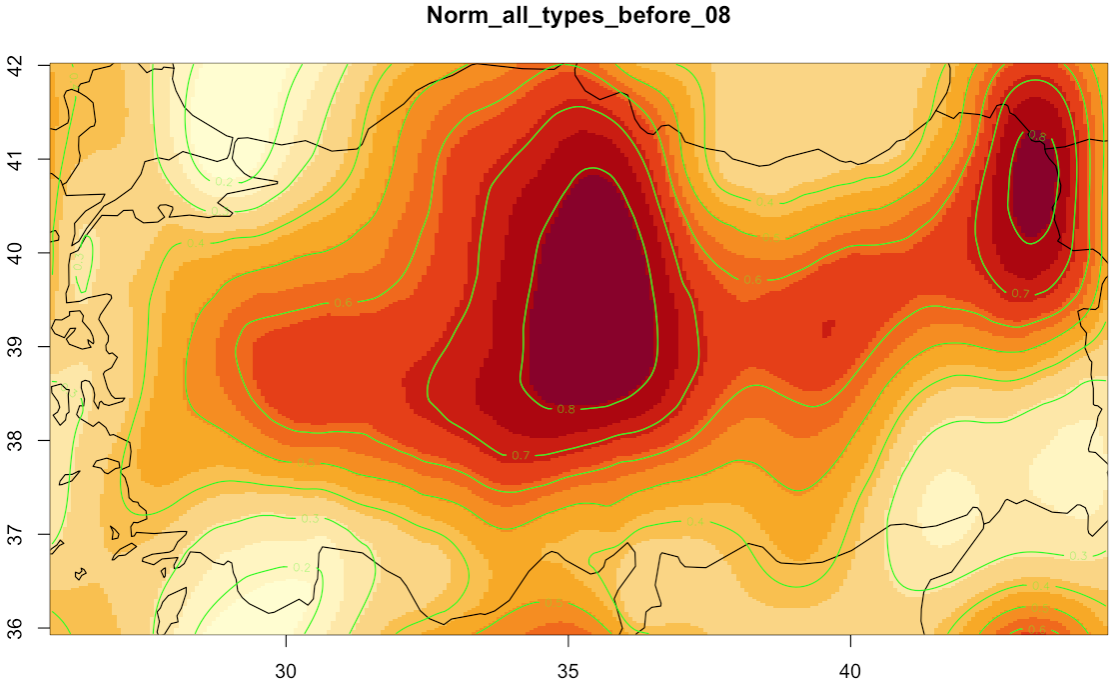}
            \caption[]{}%
            %{{\small Network 1}}    
            %\label{fig:mean and std of net14}
        \end{subfigure}
        \hfill
        \begin{subfigure}[b]{0.475\textwidth}  
            \centering 
            \includegraphics[width=\textwidth]{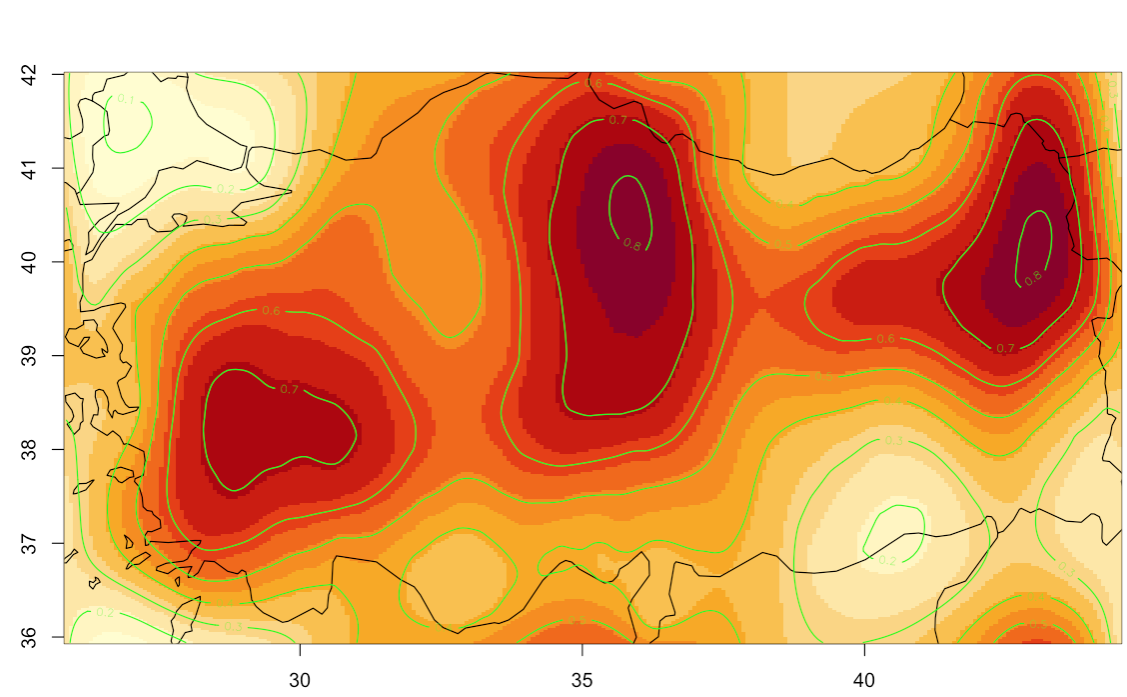}
            \caption[]{}%
           % {{\small Network 2}}    
            %\label{fig:mean and std of net24}
        \end{subfigure}
        \caption{Disease map of FMD of all types in (a) 2001-2008 (b) 2009-2012}
        \label{fig:diseasemap_time}
    \end{figure*}
    
    [[delete paragraph: should focus on time-invarying risks]] in this paper
    European and Turkish animal health officials launched a mass vaccination programme in 2008 and it is of interest to compare the relative change of susceptibility risk before and after 2008. In Figure \ref{fig:diseasemap_time} we compare the resulting risk susceptibility of in time, and noticed a decrease in the risk levels in  Thrace region which achieved FMD free as recognised by the World Organisation for Animal Health in 2010. In terms of high risk clusters, we noticed new cluster formalized in southwest while center Anatolia and northeast roughly remains being clustered. This phenomena may be relevant to the growing local livestock industry in the southwest regions instead of mainly relying on transportation from the traditional supply regions in northeast. In addition, we notice a decrease in risk levels in the southeastern boarding regions which is an achievement of enhancing  examination of livestock imported from neighboring countries.(ref 2010 Turkey Livestock Products Report, double check) ]]
